# Supplementary material for: Rust for Embedded Systems: Current State, Challenges and Open Problems (Extended Report)
Source: arXiv:2311.05063 source file (2024-09-05)
Supplement: Supplementary file 1 [file onlineresourcesback.tex]

\begin{figure*}[ht]
\centering
\scriptsize

% Is Rust Documentation helpful?
\begin{minipage}[b]{0.2\linewidth}
%\centering
%\begin{subfigure}[b][0.32\linewidth]
    
\begin{tikzpicture}
\begin{scope}[scale=0.4]
    \pie[text=inside, font=\tiny]{33.3/daddsddsds,33.3/B,33.3/A}
\end{scope}
\end{tikzpicture}
\caption{Is Documentation Helpful?}
    \label{fig:rustdochelpful}
%\end{subfigure}
\end{minipage}

%\hfill
% How can Rust Documentation be improved?
\begin{minipage}[b]{0.2\linewidth}
%\centering
\begin{tikzpicture}
\begin{scope}[scale=0.4]
    \pie[text=inside]{33.3/daddsdssa,33.3/B,33.3/A}
\end{scope}
\end{tikzpicture}
\caption{Suggestions to Improve Documentation}
    \label{fig:rustdocsuggestions}
\end{minipage}

%\hfill
% Refer external resources?
\begin{minipage}[b]{0.2\linewidth}
%\centering
\begin{tikzpicture}%
\begin{scope}[scale=0.4]
    \pie[text=inside]{33.3/daddsdssa,33.3/B,33.3/A}
\end{scope}
\end{tikzpicture}
\caption{Do you refer to external resources?}
\label{fig:rustexternalresources}
\end{minipage}

%\hfill
% Support for rust in community?
\begin{minipage}[b]{0.2\textwidth}
%\centering
\begin{tikzpicture}%
\begin{scope}[scale=0.4]
    \pie[text=inside]{33.3/daddsdssa,33.3/B,33.3/A}
\end{scope}
\end{tikzpicture}
\caption{Support for~\rust in Embedded Systems Community}
\label{fig:rustembeddeddevsupport}
\end{minipage}

\caption{Developers perspective on~\rust{} documentation and community support. \aravind{Shashank: Can you make these figures horizontally aligned.}}
\label{fig:onlineresourcesandcommunitysupport}
\Description[Developers perspective on~\rust{} documentation and community support.]{Developers perspective on~\rust{} documentation and community support.}
\end{figure*}
