# Supplementary material for: Rust for Embedded Systems: Current State, Challenges and Open Problems (Extended Report)
Source: arXiv:2311.05063 source file (2024-09-05)
Supplement: Supplementary file 2 [file rq1applicabilityappendix.tex]

\section{Applicability of Rust}
\label{apdx:applicabilityofrust}
We want to assess whether~\rust{} is a practical memory-safe language for embedded systems.
As mentioned in~\sect{subsec:embeddedsystems}, these systems have a lot of diversity in hardware (\ie~\acp{MCU}), execute in low-memory environments, and have strict timing requirements (\ie{} real-time constraints).
To assess~\rust{}'s suitability, we need to investigate: (i)~\rust{}'s existing hardware support and ease of adding new targets; (ii) Whether~\rust{} binaries are small enough to fit in a typical~\ac{MCU}, and finally, (ii) Whether the performance of~\rust{} is similar to that of native (\ie C/C++) programs.
\iffalse
Here, we want to assess whether~\rust{} is a practical memory-safe language for embedded systems.
As mentioned in~\sect{subsec:embeddedsystems}, from a software engineering perspective, these systems have the following characteristics: a lot of diversity in hardware (\ie~\acp{MCU}), execute in low-memory environments, and have strict timing requirements (\ie{} real-time constraints).
To be applicable,~\rust{} should satisfy the above requirements.
\fi

\subsection{\texorpdfstring{\rust{}'s Embedded Hardware Support}{Rust's Embedded Hardware Support}}
\label{apdx:rusthardwaresupport}

Hardware support of a compilable programming language (like~\rust{}) comprises two aspects: (i)~\ac{ISA} or Architecture support: Can the compiler generate machine instructions corresponding to the target? (ii) Target or toolchain support: Can the compiler produce a binary executable with valid instructions and data format compatible with a target processor environment?

\noindent\textbf{\ac{ISA} Support:}~\acp{MCU} use~\ac{RISC}~\acp{ISA}, such as ARM.
The~\rust{} compiler~\rustc{}~\cite{rustccompiler} uses~\llvm{} as the backend for machine code generation and consequently,~\rustc{} can also supports~\cite{rustccompilersupport} all~\acp{ISA} supported by~\llvm{}.
The recent and stable version of~\llvm,~\ie version 17, supports 36 different~\ac{RISC} architectures, including ARM, MIPS, AVR and RISC-V.
% Unfortunately,~\rustc does not have built-in support~\cite{avrrust} for AVR -- one of the common architectures in embedded systems development. However, there are active efforts~\cite{avrrust} to include this.
% \shank{ToSelf: check the latest state}.

\noindent\textbf{Target Support:}~\ac{ISA} support does not indicate that the compiler can generate a valid binary for an~\ac{MCU} with the~\ac{ISA}.
A compiler requires various other information (\eg~\ac{ABI} or calling convention) to generate an executable binary from the source code,~\lst{lst:rusttarget} shows an example of the details required to generate ARM v7 firmware. For instance, the key ``data-layout'' represents the layout of various data entities, such as stack alignment (\code{S64})).
\emph{The recent version of~\rustc{} (version: 1.70) supports 29 embedded system targets~\footnote{Computed using \shell{rustc --print target-list}}~\cite{rustcplatformsupport}, including ARM-Cortex-M, Aarch64, ARM, MSP430 --- which are the most popular and commonly used architectures in type-2 embedded systems~\cite{Scharnowski2022FuzzwareUP, 10.5555/3277203.3277227, 8835392, p2im,patterson1980case}}.

\noindent\textbf{Adding New Targets:}
Developers can add support for new targets through an architecture specification~\ie{} a JSON file with all the required information.
The~\lst{lst:rusttarget} from the Appendix shows an example of this.
%An example is shown in~\lst{lst:rusttarget} in Appendix.
Developers can use existing target specifications (using~\shell{--print target-spec-json} command) and tweak them to create new target specifications.
\iffalse
Developers can create a new target using a JSON file with all the required information, as shown in~\lst{lst:rusttarget}.
If the new target is similar to an existing target, the recommended way~\cite{creatingsustomtarget} to create the JSON is to print the existing target spec using~\shell{--print target-spec-json} command.
Second, tweaking the JSON to match the properties of the new target.
\fi

\noindent\textbf{On-going Improvements:} 
%Unfortunately,~\rustc does not have built-in support~\cite{avrrust} for AVR -- one of the common architectures in embedded systems development. However, there are active efforts~\cite{avrrust} to include this.
\gcc{} has more extensive target support for embedded systems.
There is an active effort~\gccrs{}~\cite{gccrs}, where the goal is to use integrate~\rustc{} into~\gcc{}, which also enables the use of extensive GNU tools.

\pgfplotsset{
     box plot width/.initial=1em,
     box plot/.style={
        /pgfplots/.cd,
        black,
        only marks,
        mark=-,
        mark size=\pgfkeysvalueof{/pgfplots/box plot width},
        /pgfplots/error bars/.cd,
        y dir=plus,
        y explicit,
     },
     box plot box/.style={
        /pgfplots/error bars/draw error bar/.code 2 args={%
            \draw  ##1 -- ++(\pgfkeysvalueof{/pgfplots/box plot width},0pt) |- ##2 -- ++(-\pgfkeysvalueof{/pgfplots/box plot width},0pt) |- ##1 -- cycle;
        },
        /pgfplots/table/.cd,
        y index=2,
        y error expr={\thisrowno{3}-\thisrowno{2}},
        /pgfplots/box plot
     },
     box plot top whisker/.style={
        /pgfplots/error bars/draw error bar/.code 2 args={%
            \pgfkeysgetvalue{/pgfplots/error bars/error mark}%
            {\pgfplotserrorbarsmark}%
            \pgfkeysgetvalue{/pgfplots/error bars/error mark options}%
            {\pgfplotserrorbarsmarkopts}%
            \path ##1 -- ##2;
        },
        /pgfplots/table/.cd,
        y index=4,
        y error expr={\thisrowno{2}-\thisrowno{4}},
        /pgfplots/box plot
     },
     box plot bottom whisker/.style={
        /pgfplots/error bars/draw error bar/.code 2 args={%
            \pgfkeysgetvalue{/pgfplots/error bars/error mark}%
            {\pgfplotserrorbarsmark}%
            \pgfkeysgetvalue{/pgfplots/error bars/error mark options}%
            {\pgfplotserrorbarsmarkopts}%
            \path ##1 -- ##2;
        },
        /pgfplots/table/.cd,
        y index=5,
        y error expr={\thisrowno{3}-\thisrowno{5}},
        /pgfplots/box plot
     },
     box plot median/.style={
        /pgfplots/box plot
     }
    }
\begin{figure}[h]
\centering
    \begin{tikzpicture}
    \begin{axis} [symbolic x coords={MCUs,Crn,Cre,RRTnr,RRTr}, 
    xtick=data,     
    ylabel=Size (KB),
    ylabel style={font=\footnotesize},
    ytick={0.250, 16, 256},
    %xlabel=Entities,
    xmajorgrids={true},
    height=5cm,
    width=7cm,
    axis background/.style={fill=gray!5},
    xlabel style={font=\footnotesize},
    box plot width=0.5em]
    \addplot [box plot median] table[col sep=comma] {data/sizeplotdata.txt};
     \addplot [box plot box] table[col sep=comma] {data/sizeplotdata.txt};
     \addplot [box plot top whisker] table[col sep=comma] {data/sizeplotdata.txt};
     \addplot [box plot bottom whisker] table[col sep=comma] {data/sizeplotdata.txt};
     \draw[dashed, red] (axis cs:MCUs, 16.000) -- (axis cs:RRTr, 16.000);
    \end{axis}
    \end{tikzpicture}
    \caption{Statistics of sizes of~\acp{MCU} and various~\rust{} software.}
\label{fig:mcusizeboxplot}
\Description[Statistics of sizes of~\acp{MCU} and various~\rust{} software.]{Statistics of sizes of~\acp{MCU} and various~\rust{} software.}
\end{figure}

\subsection{\texorpdfstring{Size of~\rust{} Binaries}{Size of Rust Binaries}}
\label{apdx:rustbinarysize}
Embedded systems run on~\acp{MCU} with a small amount of on-device main memory (or RAM).
We analyzed popular~\ac{MCU} boards (\apdx{apdx:macuanalysis}) and found the available memory on these devices ranges from~\minmcumemory{} bytes~\maxmcumemory{} KB.
The first bar in~\fig{fig:mcusizeboxplot} shows the box plot of memory sizes in~\ac{MCU} boards.
The red-dotted lines across show the median memory size~\ie 16KB.

One of the well-known drawbacks of~\rust is the size of the generated binary. For instance, a simple hello world program in~\rust is 4.1 MB (without debug symbols).
This large size is mainly because the standard library is automatically included in the generated binary.
We can disable this by using~\rust{}'s~\code{no_std} mode, which does not include standard libraries and other startup code.
All embedded software in~\rust{} use~\code{no_std} mode and are considerably small.
The~\rustnonembcrates{}  and~\rustembcrates{} bars in~\fig{fig:mcusizeboxplot} show the box plot of code-section sizes of non-embedded and embedded crates, respectively.
As we can see, embedded crates (\rustembcrates{}) are considerably smaller, with a median size of 10K ($<$ 16K (median MCU memory)).
Similarly, as indicated by~\nonnativerustrots{} and~\nativerustrots{} bars,~\rust{}~\acp{RTOS} are also considerably smaller with a median size of 9K and 8K, respectively.
This shows binaries produced by~\rust{} for embedded software can fit on~\ac{MCU} boards.
Furthermore, there are ongoing works~\cite{ayers2022tighten} that try to further reduce the size of~\rust{} binaries.

\subsection{\texorpdfstring{Performance of~\rust{}}{Performance of Rust}}
\label{apdx:rustperf}
Several works compare the performance of~\rust{} programs with those written in C/C++.
The results are contradictory.
Few works~\cite{rustvsc,spedofrust} show that~\rust{} programs are as fast or even faster than C/C++ counterparts.
However, recently Zhang~\etal{}~\cite{junperformance} argue that~\rust{} programs are consistently slower.
Furthermore, the conclusions of these studies change as~\rustc evolves with more optimizations.

The main reasons for performance overhead (if any) in~\rust{} is because of using~\texttt{std} library and additional runtime checks.
However, embedded software in~\rust{} is compiled with~\code{no_std} mode, which does not include ~\texttt{std} library and has all many checks disabled~\cite{rustonmicro}.
Several~\rust{} based~\acp{RTOS} are developed (\sect{apdx:rustbinarysize}) based on this and have performance comparable to traditional~\acp{RTOS}.
However,~\emph{no existing study systematically tries to evaluate~\rust{}'s performance on embedded systems}.

\begin{tcolorbox} [width=\linewidth, colback=yellow!30!white, top=1pt, bottom=1pt, left=2pt, right=2pt]
\textbf{Finding App.1 (\ref{apdx:rusthardwaresupport}):} 
The architecture support by~\rust{} is adequate for embedded systems.
Although AVR is not readily supported, there are promising ongoing efforts to improve this.

\textbf{Finding App.2 (\ref{apdx:rustbinarysize}):}
\rust{}'s~\code{no_std} mode enables generation of smaller binaries which can fit into most~\acp{MCU} memory.
 
\textbf{Finding App.3 (\ref{apdx:rustperf}):}
There are high-performant configurations (\code{no_std}) of~\rust{}, which results in performance similar to that of native programs. However, no work exists that tries to do a systematic performance evaluation of~\rust{} embedded systems.

\end{tcolorbox}
